# Supplementary material for: GR-MG: Leveraging Partially Annotated Data via Multi-Modal Goal-Conditioned Policy
Source: arXiv:2408.14368 source file (2024-12-23)
Supplement: Supplementary file 1 [file appendix.tex]

\raggedcolumns 
\begin{table}[]
\centering
\caption{Data Hyperparameters}
\resizebox{\columnwidth}{!}{%
\begin{tabular}{@{}ccccc@{}}
\toprule
     & CALVIN~\cite{mees2022calvin} & SSV2~\cite{goyal2017something} & RT-1~\cite{brohan2022rt} &  Real \\ \midrule
$k_\mathrm{min}$ & 20     & 11                     & 5    & 30       \\
$k_\mathrm{max}$ & 22     & 14                     & 6    & 35       \\
% $k_{n}$   & 1      & 5                      & 3    & 5        \\ 
$h$   & 10      & -                      & -    & 7        \\
$k_\mathrm{act}$   & 5      & -                      & -    & 15        \\
$k_\mathrm{pmax}$   & 25      & -                      & -    & 35        \\
% $k_{pred}$   & 3      & N/A                      & N/A    & 3        \\ 
\bottomrule
\end{tabular}
}
\label{tab:sample_interval}
\end{table}

\subsection{Data}
To train the goal generation model, we resize all images to 256$\times$256 before encoding.
Additionally, we sample a ground truth goal image from future frames within a range defined by $k_\mathrm{min}$ and $k_\mathrm{max}$. 
The values for different datasets are listed in Tab.~\ref{tab:sample_interval}. 
We sample tuples of ($l$, $o_t$, $o_{t+k}$, $p$) for training, where $l$ represents the language instruction, $o_{t}$ is the current observation, $o_{t+h}$ is the target goal image, and $p$ indicates the progress information.
$p$ is computed from the timestep of the input image in the video.

To train the policy, all images are resized to 224$\times$224 to match the input requirements of the MAE~\cite{he2022masked} encoder.
The policy takes $h$ steps of observation history as input and outputs an action trajectory of $k_\mathrm{act}$ steps. 
Groundtruth goal images are sampled from future frames within the trajectory.
Specifically, we sample an image from the next step up to the next $k_\mathrm{pmax}$-th step. 
Similar to GR-1~\cite{wu2023unleashing}, we train the policy to predict both actions and future images.
We set the target future image as the next 3rd frame. 
See Table \ref{tab:sample_interval} for more details.

\subsection{Progress-guided Goal Image Generation Model}
The progress-guided goal image generation model is based on InstructPix2Pix~\cite{brooks2023instructpix2pix}. 
The goal image generation is performed via a diffusion process in the latent space defined by a VAE image encoder~\cite{kingma2013auto}. 
Firstly, the input image is encoded into a latent representation by the VAE encoder. 
Secondly, the U-Net denoises the latent features conditioned on the input image and the text.
The text condition is injected via cross-attention. 
Finally, the denoised latent features are decoded by the VAE decoder to produce the goal image. 
We employ classifier-free guidance~\cite{ho2022classifier} during the diffusion process.
We set the number of denoising steps as 50 during inference.

\begin{table}[]
\centering
\caption{Training Hyperparameters}
\resizebox{\columnwidth}{!}{%
\begin{tabular}{@{}ccc@{}}
\toprule
& {Goal Image} & {Multi-Modal Goal}   \\
& {Generation Model} & {Conditioned Policy} \\
\midrule
{batch size}    & {1024} & {512}      \\
{learning rate} & {8e-5} & {1e-3} \\
{optimizer}     & {AdamW} & {AdamW} \\
{weight decay}  & {1e-2} & {0} \\
{adam\_beta1}   & {0.95} & {0.9}      \\
{adam\_beta2}   & {0.999}& {0.999}    \\
{epoch}         & {50}   & {50}       \\ 
\bottomrule
\end{tabular}
}
\label{tab:training_hyper}
\end{table}

\subsection{Multi-modal Goal Conditioned Policy}
For the multi-modal goal-conditioned policy, each image is first encoded into 196 patch tokens and one global token corresponding to the output of the input \texttt{[CLS]} token.
The 196 patch tokens are then reduced to 9 tokens with a Perceiver Resampler~\cite{alayrac2022flamingo}.
We use CLIP~\cite{radford2021learning} to encode the language instruction.
Robot states are encoded via linear layers.
Before inputting the tokens to the GPT model, we use linear layers to align the dimension of all tokens to the hidden size of the GPT model.
The hidden size, number of heads, and number of layers for the GPT model is 384, 12, and 12, respectively.
We follow~\cite{zhao2023learning} to predict the action trajectory via a cVAE~\cite{kingma2013auto,sohn2015learning}.
\subsection{Training}
Our goal image generation model is trained on 16 NVIDIA A100 GPUs (80GB) for 50 epochs. 
Training takes approximately 18 hours on the CALVIN Benchmark and about 30 hours in the real-robot experiments. 
During training, we apply data augmentation using CenterCrop and ColorJitter. 
Additionally, we find that using an Exponential Moving Average (EMA) is crucial for stabilizing the performance of GR-MG.

We train the policy on 32 NVIDIA A800 GPUs (40GB) for 50 epochs, which takes about 17 hours for the CALVIN Benchmark and 7 hours for the real-robot experiments. 
The training loss consists of five components: arm action prediction loss \(l_\mathrm{arm}\), gripper action prediction loss \(l_\mathrm{gripper}\), future image prediction loss \(l_\mathrm{img}\), KL divergence loss from VAE \(l_\mathrm{kl}\)~\cite{zhao2023learning}, and progress loss \(l_\mathrm{prog}\):
\begin{equation}
    L = l_\mathrm{arm} + 0.01 l_\mathrm{gripper} + 0.1 l_\mathrm{img} + l_\mathrm{kl} + l_\mathrm{prog}
    \label{eq:1}
\end{equation}
We list the training hyperparameters in Table \ref{tab:training_hyper}.
